# Supplementary material for: SMCQL: Secure Querying for Federated Databases
Source: arXiv:1606.06808 source file (2017-03-06)
Supplement: Supplementary file 1 [file appendix.tex]

\appendix
\section{Secure Multiparty Computation} 
\label{sec:background-smc}

%Similarly, for if-then statements, a SMC program must execute both branches of the statement in order to stay oblivious to the values in the input data.

%To prevent information leaks, the PDN architecture has a security policy so that the honest broker controls the conditions under which a query is admitted for execution.

In Figure~\ref{fig:garbled-circuit}, we show an example of a garbled circuit with a single OR gate.  Each garbled gate has two main ingredients: keyed wire labels and a garbled truth table.  The first party, Alice,  generates the garbled circuit by creating secret keys that represent each possible value for each wire in the gate.   She then translates the original gate's truth table into one using the keys as displayed in Figure~\ref{fig:garbled-circuit-after}.  After that, she creates a list of garbled values based on the truth table for sharing with Bob.  Each garbled value contains a one-way hash over the two input keys combined with the gate ID, $g_0$.  The gate ID is a secure nonce that prevents values from repeating in a multi-gate circuit.   This hashed value is XORed with the value of the output wire associated with this key combination.   
\begin{figure}[t!]
\centering
\resizebox{.5\textwidth}{!}{%
\begin{tikzpicture}[circuit logic US]
      
\node[or gate, minimum height = 15mm] (or1)   {$g_0$};
 \node[right=4cm of or1, or gate, minimum height = 15mm] (or2) {$g_0$};
 %   \node[right=of or1, or gate, point up] (or2)  {};
 
 \draw (or1.output)  -- ++(right:5mm) node [right]{$w_2$};   
  	\draw ($(or1.input 1) + (-0.75mm, 1.5mm)$)-- ++(left:5mm) node [left]{ $w_0$};
    \draw ($(or1.input 2) + ( -0.75mm, -1.5mm)$)-- ++(left:5mm) node [left]{$w_1$};
 
 \draw (or2.output)  -- ++(right:5mm) node [right]{$\{k_0^2, k_1^2 \}$};   
  	\draw ($(or2.input 1) + (-0.75mm, 1.5mm)$)-- ++(left:5mm) node [left]{ $\{ k_0^0, k_1^0 \}$};
    \draw ($(or2.input 2) + ( -0.75mm, -1.5mm)$)-- ++(left:5mm) node [left]{ $ \{ k_0^1, k_1^1\}$};
 
  \end{tikzpicture}
}
\end{figure}

\begin{figure}
	
\begin{subfigure}[t]{.2\textwidth}
\centering
\begin{tabular}{ c| c |c }
$w_0$ & $w_1$ & $w_2$\\
\hline
0 & 0 & 0\\
0 & 1 & 1 \\
1 & 0 & 1 \\
1 & 1 & 1 \\
\end{tabular}
\caption{Initial gate.}
\label{fig:garbled-circuit-before}
\end{subfigure}%
~
\begin{subfigure}[t]{.3\textwidth}
\centering
\begin{tabular}{ c| c |c |c}
$w_0$ & $w_1$ & $w_2$ & Garbled Value \\
\hline
$k_0^0$ & $k_0^1$ & $k_0^2$ & $H(k_0^0||k_0^1||g_0) \oplus k_0^2$\\
$k_0^0$ & $k_1^1$ & $k_1^2$  & $H(k_0^0||k_1^1||g_0) \oplus k_1^2$\\
$k_1^0$ & $k_0^1$ & $k_1^2$ & $H(k_1^0||k_0^1||g_0) \oplus k_1^2$\\
$k_1^0$ & $k_1^1$ & $k_1^2$  & $H(k_1^0||k_1^1||g_0) \oplus k_1^2$\\
\end{tabular}
\caption{Garbled gate.}
\label{fig:garbled-circuit-after}
\end{subfigure}
\caption{Example of garbling an OR gate.}
\label{fig:garbled-circuit}
\end{figure}

Alice sends the garbled gate to Bob for evaluation.  Thus he can see all six keys, $k_i^j$, but he does not know the true values associated with each one.  She also ships the four garbled values to him after randomizing their order so that he cannot guess their position in the truth table.   In addition, Alice sends her input to the garbled circuit, $k^a \in \{k_0^0, k_1^0\}$.  After that, Bob determines his input key using OT.   At the end of this step, he has $k^b \in  \{k_0^1, k_1^1\}$ and has not seen the other possible key for this wire.  

Now Bob solves for the output of this circuit.  Recall that if we XOR a value with itself, the result  is always equal to zero.  Thus if we calculate $H\oplus k \oplus H$, it will produce $k$.  Bob calculates $H(k^a || k^b || g_0)$ and XORs it with each of the four garbled values in Figure~\ref{fig:garbled-circuit-after}.  The matching garbled value will produce either $k_0^2$ or $k_1^2$, and the others result in $\perp$. Bob has no way of relating this key to its plaintext value.   This is the output of the garbled circuit for $w_2$. 

If the circuit contained more gates, Bob would use $w_2$'s key as input to the next gate in the circuit.  The next gate would come with its own set of hashed garbled values and Bob would continue to solve for subsequent output labels.  See~\cite{Dokos2014, snyderyao} for a more detailed introduction to garbled circuits. 

At the end of the circuit, Bob sends his output key(s) to a neutral third-party honest broker over an encrypted connection.  Alice reports the true labels associated with the output keys to the honest broker using a separate secure connection.  The honest broker compares Bob's output to the ones provided by Alice and records the plaintext result of the circuit.  Note that at the end of this neither Alice nor Bob has access to the unencrypted output of the garbled circuit.

%For boolean circuits such as ours, the garbled function is computed on, and produces, one or more {\it shared secret bits} (SSBs) or boolean labels.  Thus at the beginning of a circuit, each party selects one of two SSBs to denote whether their input bit is zero or one.  The parties determine their inputs using {\it oblivious transfer}.  Here, the sender (Alice) has two SSB labels, $s_0$ and $s_1$, and the receiver (Bob) has a bit $b$.  Bob wants access to $s_b$, without disclosing $b$ to Alice.  At the same time, Alice  wants to ensure that the receiver receives only one of the two labels.  The output of a garbled circuit is another SSB, computed based on the inputs selected by oblivious transfer.   Taken alone by each party, each output SSB has no intrinsic meaning.  If we combine the SSBs of Alice and Bob as the output of a SMC function, we produce the plaintext result of the computation.  See~\cite{Dokos2014, snyderyao} for more background on garbled circuits.  In our setting, we permit neither Alice nor Bob to put together two halves of the shared secrets produced by a {\sc \sysname} query. Instead, only the honest broker accesses the plaintext results of a SMC function.
